# Supplementary material for: DIPPA: An improved Method for Bilinear Saddle Point Problems
Source: arXiv:2103.08270 source file (2021-03-15)
Supplement: Supplementary file 2 [file apfb.tex]

\section{Proof of Theorem \ref{thm:apfb}}
\label{app:apfb}
\begin{proof}
    Note that 
    \begin{align*}
        \vy_k = \argmin_{\vy} H_k(\vy) \triangleq h(\vy) + \frac{1}{2 \sigma} \norm{\vy - \vy_{k-1} - \sigma \mA^{\top} \tilde\vx_{k-1}}^2.
    \end{align*}
    By $(\mu_y + 1/\sigma)$-strongly convexity of $H_k$, we know that
    \begin{align*}
        &\quad h(\vy^*) + \frac{1}{2\sigma} \norm{\vy^* - \vy_{k-1} - \sigma \mA^{\top} \tilde\vx_{k-1}}^2 \\
        &\ge h(\vy_k) + \frac{1}{2\sigma} \norm{\vy_k - \vy_{k-1} - \sigma \mA^{\top} \tilde\vx_{k-1}}^2 + \left( \frac{\mu_y}{2} + \frac{1}{2\sigma}\right) \norm{\vy_k - \vy^*}^2,
    \end{align*}
    that is 
    \begin{align}
        \notag &\quad h(\vy^*) + \frac{1}{2\sigma} \norm{\vy_{k-1} - \vy^*}^2 + \inner{\vy_k - \vy^*}{\mA^{\top} \tilde\vx_{k-1}} \\
        \label{apfb:proof:1} &\ge h(\vy_k) + \frac{1}{2\sigma} \norm{\vy_k - \vy_{k-1}}^2 + \left( \frac{\mu_y}{2} + \frac{1}{2\sigma}\right) \norm{\vy_k - \vy^*}^2.
    \end{align}
    
    Similarly, by 
    \begin{align*}
        \vx_k = \argmin_{\vx} g(\vx) + \frac{1}{2 \gamma} \norm{\vx - \vx_{k-1} + \gamma \mA \vy_{k}}^2,
    \end{align*}
    we have
    \begin{align*}
        &\quad g(\vx^*) + \frac{1}{2\gamma} \norm{\vx^* - \vx_{k-1} + \gamma \mA \vy_k}^2 \\
        &\ge g(\vx_k) + \frac{1}{2\gamma} \norm{\vx_k - \vx_{k-1} + \gamma \mA \vy_k}^2 + \left( \frac{\mu_x}{2} + \frac{1}{2\gamma}\right) \norm{\vx_k - \vx^*}^2,
    \end{align*}
    which implies 
    \begin{align}
        \notag &\quad g(\vx^*) + \frac{1}{2\gamma} \norm{\vx_{k-1} - \vx^*}^2 - \inner{\vx_k - \vx^*}{\mA \vy_k} \\
        \label{apfb:proof:2} &\ge g(\vx_k) + \frac{1}{2\gamma} \norm{\vx_k - \vx_{k-1}}^2 + \left( \frac{\mu_x}{2} + \frac{1}{2\gamma}\right) \norm{\vx_k - \vx^*}^2.
    \end{align}
    
    Then we add both sides of the inequalities (\ref{apfb:proof:1}) and (\ref{apfb:proof:2}). Thus we have
    \begin{equation}\label{apfb:proof:3}
    \begin{aligned}
        &\quad \frac{1}{2\gamma} \norm{\vx_{k-1} - \vx^*}^2 + \frac{1}{2\sigma} \norm{\vy_{k-1} - \vy^*}^2 \\
        &\ge \left( \frac{\mu_x}{2} + \frac{1}{2\gamma}\right) \norm{\vx_k - \vx^*}^2 + \left( \frac{\mu_y}{2} + \frac{1}{2\sigma}\right) \norm{\vy_k - \vy^*}^2 \\
        &\quad + \frac{1}{2\gamma} \norm{\vx_k - \vx_{k-1}}^2 + \frac{1}{2\sigma} \norm{\vy_k - \vy_{k-1}}^2 \\
        &\quad + g(\vx_k) + h(\vy_k) - g(\vx^*) - h(\vy^*) + \inner{\vx_k - \vx^*}{\mA \vy_k} - \inner{\vy_k - \vy^*}{\mA^{\top} \tilde\vx_{k-1}}.
    \end{aligned}
    \end{equation}
    
    Observe that
    \begin{align}\label{apfb:proof:4}
        f(\vx_k, \vy^*) - f(\vx^*, \vy_k) 
        = g(\vx_k) + \inner{\vx_k}{\mA \vy^*} - h(\vy^*) - g(\vx^*) - \inner{\vx^*}{\mA \vy_k} + h(\vy_k).
    \end{align}
    Plugging Equality (\ref{apfb:proof:4}) into Inequality (\ref{apfb:proof:3}), we have
    \begin{equation}\label{apfb:proof:5}
    \begin{aligned}
        &\quad \frac{1}{2\gamma} \norm{\vx_{k-1} - \vx^*}^2 + \frac{1}{2\sigma} \norm{\vy_{k-1} - \vy^*}^2 \\
        &\ge \left( \frac{\mu_x}{2} + \frac{1}{2\gamma}\right) \norm{\vx_k - \vx^*}^2 + \left( \frac{\mu_y}{2} + \frac{1}{2\sigma}\right) \norm{\vy_k - \vy^*}^2 
        + \frac{1}{2\gamma} \norm{\vx_k - \vx_{k-1}}^2 + \frac{1}{2\sigma} \norm{\vy_k - \vy_{k-1}}^2 \\
        &\quad + f(\vx_k, \vy^*) - f(\vx^*, \vy_k) + \inner{\vx_k - \tilde\vx_{k-1}}{\mA (\vy_k - \vy^*)}.
        % &\ge \left( \frac{\mu_x}{2} + \frac{1}{2\gamma}\right) \norm{\vx_k - \vx^*}^2 + \left( \frac{\mu_y}{2} + \frac{1}{2\sigma}\right) \norm{\vy_k - \vy^*}^2 
        % + \frac{1}{2\gamma} \norm{\vx_k - \vx_{k-1}}^2 + \frac{1}{2\sigma} \norm{\vy_k - \vy_{k-1}}^2 \\
        % &\quad + \inner{\vx_k - \vx_{k-1} - \theta (\vx_{k-1} - \vx_{k-2})}{\vy_k - \vy^*}.
    \end{aligned}
    \end{equation}
    
    With recalling the definition of $\tilde\vx_{k-1}$, the last term of Inequality (\ref{apfb:proof:5}) can be rewritten as
    \begin{equation}\label{apfb:proof:6}
    \begin{aligned}
        &\quad \inner{\vx_k - \tilde\vx_{k-1}}{\mA (\vy_k - \vy^*)} \\
        &= \inner{\vx_k - \vx_{k-1} - \theta (\vx_{k-1} - \vx_{k-2})}{\mA(\vy_k - \vy^*)} \\
        &= \inner{\vx_k - \vx_{k-1}}{\mA(\vy_k - \vy^*)} - \theta \inner{\vx_{k-1} - \vx_{k-2}}{\mA(\vy_{k-1} - \vy^*)} - \theta \inner{\vx_{k-1} - \vx_{k-2}}{\mA(\vy_k - \vy_{k-1})}.
    \end{aligned}
    \end{equation}
    
    Furthermore, we have
    \begin{equation}\label{apfb:proof:7}
    \begin{aligned}
        &\quad - \theta \inner{\vx_{k-1} - \vx_{k-2}}{\mA(\vy_k - \vy_{k-1})} \\
        &\ge -\theta \norm{\mA} \norm{\vx_{k-1} - \vx_{k-2}} \norm{\vy_k - \vy_{k-1}} \\
        &\ge -\frac{\theta}{2} \norm{\mA} \sqrt{\frac{\mu_x}{\mu_y}} \norm{\vx_{k-1} - \vx_{k-2}}^2 -\frac{\theta}{2} \norm{\mA} \sqrt{\frac{\mu_y}{\mu_x}} \norm{\vy_k - \vy_{k-1}}^2 \\
        &\ge - \frac{\theta}{2\gamma}\norm{\vx_{k-1} - \vx_{k-2}}^2 - \frac{1}{2\sigma} \norm{\vy_k - \vy_{k-1}}^2,
    \end{aligned}
    \end{equation}
    where we have recalled that $\gamma = \frac{1}{\norm{\mA}} \sqrt{\frac{\mu_y}{\mu_x}}, \sigma = \frac{1}{\norm{\mA}} \sqrt{\frac{\mu_x}{\mu_y}}$ and $\theta < 1$. 
    Similarly, there also holds
    \begin{align}\label{apfb:proof:8}
        \inner{\vx_k - \vx_{k-1}}{\mA(\vy_k - \vy^*)} \ge - \frac{1}{2\gamma} \norm{\vx_k - \vx_{k-1}}^2 - \frac{1}{2\sigma} \norm{\vy_k - \vy^*}^2.
    \end{align}
    
    Plugging Equation (\ref{apfb:proof:6}) and (\ref{apfb:proof:7}) into Inequality (\ref{apfb:proof:5}), we know that
    \begin{align*}
        &\quad \frac{1}{2\gamma} \norm{\vx_{k-1} - \vx^*}^2 + \frac{1}{2\sigma} \norm{\vy_{k-1} - \vy^*}^2 + \frac{\theta}{2\gamma}\norm{\vx_{k-1} - \vx_{k-2}}^2 + \theta \inner{\vx_{k-1} - \vx_{k-2}}{\mA(\vy_{k-1} - \vy^*)} \\
        &\ge \left( \frac{\mu_x}{2} + \frac{1}{2\gamma}\right) \norm{\vx_k - \vx^*}^2 + \left( \frac{\mu_y}{2} + \frac{1}{2\sigma}\right) \norm{\vy_k - \vy^*}^2 
        + \frac{1}{2\gamma} \norm{\vx_k - \vx_{k-1}}^2 \\
        &\quad + f(\vx_k, \vy^*) - f(\vx^*, \vy_k) + \inner{\vx_k - \vx_{k-1}}{\mA(\vy_k - \vy^*)}. 
    \end{align*}

    Therefore we have
    \begin{align*}
        &\quad \frac{\mu_x}{2} \norm{\vx_k - \vx^*}^2 + \frac{\mu_y}{2} \norm{\vy_k - \vy^*}^2 \\
        &\le \left( \frac{\mu_x}{2} + \frac{1}{2\gamma}\right) \norm{\vx_k - \vx^*}^2 + \left( \frac{\mu_y}{2} + \frac{1}{2\sigma}\right) \norm{\vy_k - \vy^*}^2 
        + \frac{1}{2\gamma} \norm{\vx_k - \vx_{k-1}}^2 + \inner{\vx_k - \vx_{k-1}}{\mA(\vy_k - \vy^*)} \\
        &\le \theta^{k} \left( \left( \frac{\mu_x}{2} + \frac{1}{2\gamma}\right) \norm{\vx_0 - \vx^*}^2 + \left( \frac{\mu_y}{2} + \frac{1}{2\sigma}\right) \norm{\vy_0 - \vy^*}^2 \right) \\
        &= \frac{\norm{\mA} \theta^{k-1} }{2}  \left( \sqrt{\frac{\mu_x}{\mu_y}}\norm{\vx_0 - \vx^*}^2 + \sqrt{\frac{\mu_y}{\mu_x}}\norm{\vy_0 - \vy^*}^2  \right).
    \end{align*}
\end{proof}
