# Supplementary material for: DIPPA: An improved Method for Bilinear Saddle Point Problems
Source: arXiv:2103.08270 source file (2021-03-15)
Supplement: Supplementary file 4 [file dppa.tex]

\section{Proof of Theorem \ref{thm:dppa}}
\begin{proof}
    Since $(\vx^*, \vy^*)$ is the saddle point of $f$, there holds $\nabla f(\vx, \vy) = 0$, that is 
    \begin{equation}\label{eq:dppa:saddle}
    \begin{aligned}
        \nabla g(\vx^*) + \mA \vy^* = 0, ~~~
        \nabla h(\vy^*) - \mA^{\top} \vx^* = 0.
    \end{aligned}
    \end{equation}
    Note that $(\vx_k, \vy_k) = \prox_{\alpha \mA} (2 \tilde\vx_k - \vz_k, 2\tilde\vy_k - \vw_k)$ which implies that
    \begin{align*}
        (\vx_k, \vy_k) = \arg\min_{\vx}\max_{\vy} \tilde{f}_k(\vx, \vy) \triangleq \frac{1}{2} \norm{\vx - 2 \tilde\vx_k + \vz_k}^2 - \frac{1}{2} \norm{\vy - 2\tilde\vy_k + \vw_k} + \inner{\vx}{\mA \vy}.
    \end{align*}
    % Letting the gradient of $\tilde{f}_k$ equal to zero, we have
    Hence, we have $\nabla \tilde{f}_k (\vx_k, \vy_k) = 0$, that is 
    \begin{equation}\label{eq:dppa:prox2}
    \begin{aligned}
        \vx_k - (2 \tilde\vx_k - \vz_k) + \alpha \mA \vy_k = 0, \\
        \vy_k - (2\tilde\vy_k - \vw_k) - \alpha \mA^{\top} \vx_k = 0.
    \end{aligned}
    \end{equation}
    Similarly, according to $(\tilde\vx_k, \tilde\vy_k) = \prox_{\alpha (g - h)}(\vz_k, \vw_k)$, we have
    \begin{equation}\label{eq:dppa:prox1}
    \begin{aligned}
        \alpha \nabla g(\tilde\vx_k) + \tilde\vx_k - \vz_k = 0, \\
        \alpha \nabla h(\tilde\vy_k) + \tilde\vy_k - \vw_k = 0.
    \end{aligned}
    \end{equation}
    
    Therefore, we can conclude that 
    \begin{align*}
        &\quad \norm{\vz_{k+1} - \vz^*}^2 + \norm{\vw_{k+1} - \vw^*}^2 \\
        &= \norm{\vx_k - \vx^* - \alpha \mA (\vy_k - \vy^*)}^2 + \norm{\vy_k - \vy^* + \alpha \mA^{\top} (\vx_k - \vx^*)}^2 \\
        &= \norm{\vx_k - \vx^*}^2 + \norm{\vy_k - \vy^*}^2 + \alpha^2 \norm{\mA (\vy_k - \vy^*)}^2 + \alpha^2 \norm{\mA^{\top} (\vx_k - \vx^*)}^2 \\
        &= \norm{\vx_k - \vx^* + \alpha \mA (\vy_k - \vy^*)}^2 + \norm{\vy_k - \vy^* - \alpha \mA^{\top} (\vx_k - \vx^*)}^2 \\
        &= \norm{2 \tilde\vx_k - \vz_k -\vx^* - \alpha \mA \vy^* }^2 + \norm{2 \tilde\vy_k - \vw_k - \vy^* + \alpha \mA^{\top} \vx^*}^2 \\
        &= \norm{\tilde\vx_k - \alpha \nabla g(\tilde\vx_k) - \vx^* + \alpha \nabla g(\vx^*)}^2 + \norm{\tilde\vy_k - \alpha \nabla h(\tilde\vy_k) - \vy^* + \alpha \nabla h(\vy^*)}^2,
    \end{align*}
    where the forth equality is based on Equation (\ref{eq:dppa:prox2}) and the last equality follows from Equation (\ref{eq:dppa:saddle}) and (\ref{eq:dppa:prox1}). 
    
    On the other hand, by Equation (\ref{eq:dppa:saddle}) and (\ref{eq:dppa:prox1}), we also have
    \begin{align*}
        \norm{\vz_{k} - \vz^*}^2 + \norm{\vw_{k} - \vw^*}^2 
        = \norm{\tilde\vx_k + \alpha \nabla g(\tilde\vx_k) - \vx^* - \alpha \nabla g(\vx^*)}^2 + \norm{\tilde\vy_k + \alpha \nabla h(\tilde\vy_k) - \vy^* - \alpha \nabla h(\vy^*)}^2
    \end{align*}
    
    Now, We only need to prove that 
    \begin{align}\label{dppa:proof}
        \norm{\tilde\vx_k - \alpha \nabla g(\tilde\vx_k) - \vx^* + \alpha \nabla g(\vx^*)}^2 \le \eta \norm{\tilde\vx_k + \alpha \nabla g(\tilde\vx_k) - \vx^* - \alpha \nabla g(\vx^*)}^2.
    \end{align}
    In fact, above inequality is equivalent to 
    \begin{align}\label{dppa:proof:2}
        (1 - \eta) \left(\norm{\tilde\vx_k - \vx^*}^2 + \alpha^2 \norm{\nabla g(\tilde\vx_k) - \nabla g(\vx^*)}^2 \right) 
        \le 2(1 + \eta)\alpha \inner{\tilde\vx_k - \vx^*}{\nabla g(\tilde\vx_k) - \nabla g(\vx^*)}.
    \end{align}
    Recalling the definition of $\eta$, we have $\frac{1 - \eta}{2(1 + \eta)} = \frac{\sqrt{L \mu}}{L + \mu}$. 
    Then together with $\alpha = 1/\sqrt{L \mu}$, inequality (\ref{dppa:proof:2}) is just
    \begin{align*}
        \frac{L \mu}{L + \mu} \norm{\tilde\vx_k - \vx^*}^2 + \frac{1}{L + \mu} \norm{\nabla g(\tilde\vx_k) - \nabla g(\vx^*)}^2 \le \inner{\tilde\vx_k - \vx^*}{\nabla g(\tilde\vx_k) - \nabla g(\vx^*)},
    \end{align*}
    which holds according to Lemma \ref{lem:smooth}.
    \end{proof}
    
\begin{remark}
    By the proof of inequality (\ref{dppa:proof}), there also holds
    \begin{align}\label{eq:dppa:3}
        \norm{2 \tilde\vx_k - \vz_k - 2 \vx^* + \vz^* }^2 \le \eta \norm{\vz_{k} - \vz^*}^2.
    \end{align}
\end{remark}
